# Supplementary material for: User-centric evaluation of explainability of AI with and for humans: a comprehensive empirical study
Source: arXiv:2410.15952 source file (2024-10-21)
Supplement: Supplementary file 1 [file slides.pdf]

Celem tego badania jest zastosowanie technik Objaśnialnej Sztucznej Inteligencji (XAI) do analizy danych dotyczących grzybów. XAI pozwala na zrozumienie, jak modele sztucznej inteligencji, takie jak klasyfikatory, podejmują decyzje. Jest to szczególnie ważne w dziedzinach, w których dokładność i wiarygodność predykcji są kluczowe, jak w przypadku odróżniania grzybów jadalnych od trujących.

Za chwilę będziemy Państwa prosić o zinterpretowanie kilku wizualizacji (głównie wykresów), które pokazują, w jaki sposób sztuczna inteligencja (AI) przewiduje, że grzyb dziko rosnący, mający określone cechy, jest albo jadalny, albo niejadalny lub trujący.

Wyjściowy zbiór danych, na którym pracowała AI, pochodzi z UC Irvine Machine Learning Repository, czyli biblioteki ćwiczebnych zbiorów danych Uniwersytetu Kalifornijskiego w Irvine, przeznaczonych do trenowania (doskonalenia) algorytmów uczenia maszynowego.

Link do tego zbioru:
https://archive.ics.uci.edu/dataset/848/secondary+mushroom+dataset

Zbiór danych („dataset”) zawiera informacje o 61 069 owocnikach 173 gatunków grzybów sklasyfikowanych jako jadalne albo niejadalne lub trujące. Grzyby o nieznanej jadalności zostały zaliczone do niejadalnych lub trujących.

**Są to wyłącznie grzyby kapeluszowe mające trzon i hymenofor blaszkowy.**

Część danych to dane symulacyjne, hipotetyczne, czyli sztucznie wygenerowane na podstawie mniejszego zbioru rzeczywistych obserwacji grzybów występujących w przyrodzie.

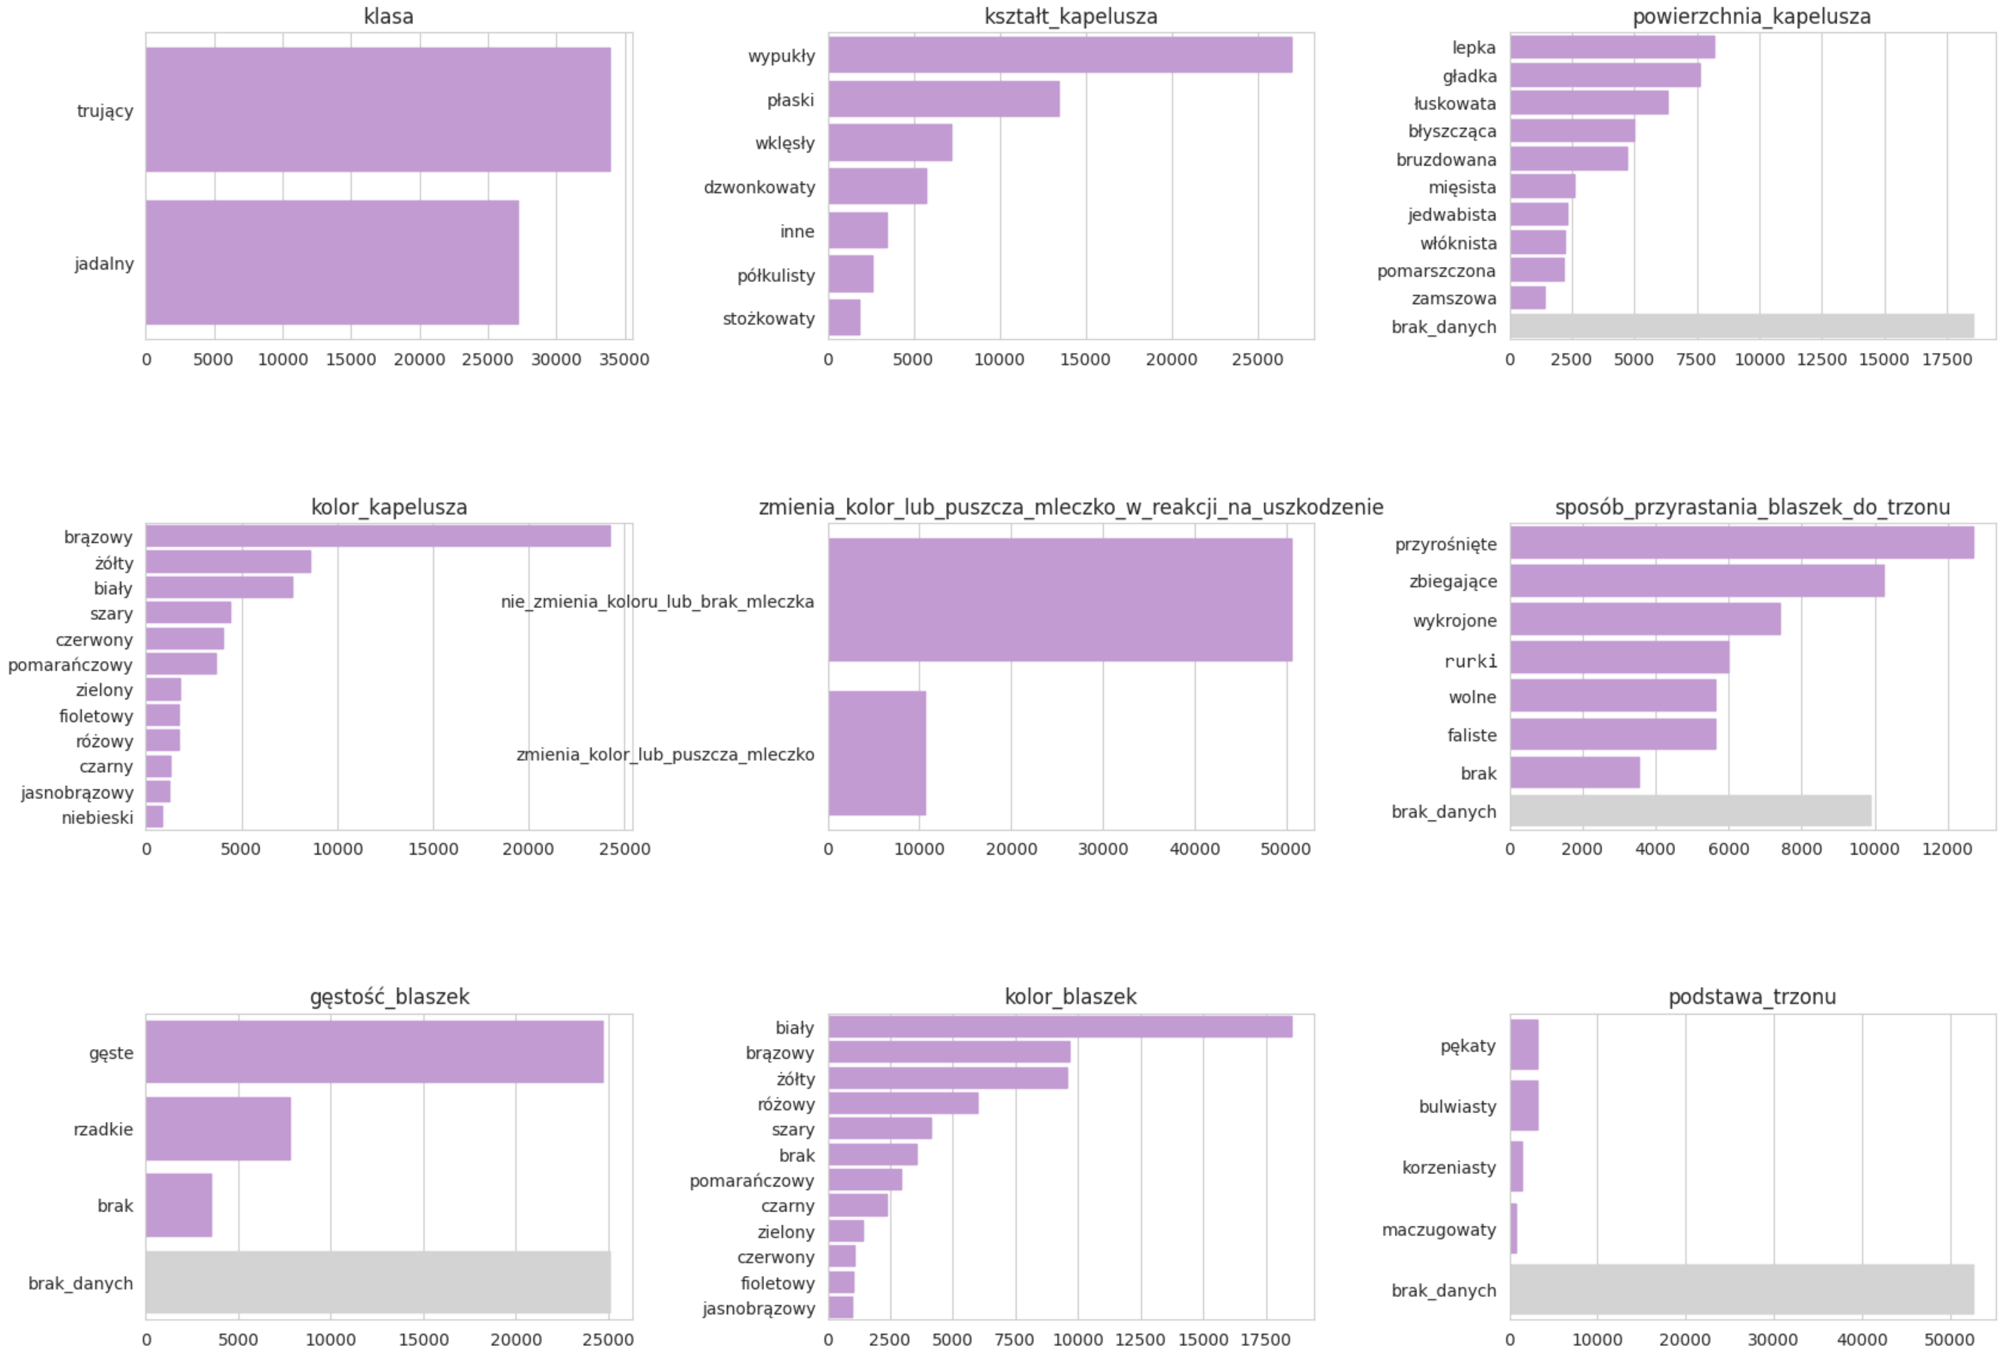
klasa
trujący
jadalny
0
5000
10000
15000
20000
25000
30000
35000
kształt_kapelusza
wypukły
płaski
wklęsły
dzwonkowaty
inne
półkulisty
stożkowaty
0
5000
10000
15000
20000
25000
powierzchnia_kapelusza
lepka
gładka
łuskowata
błyszcząca
bruzdowana
mięsista
jedwabista
włóknista
pomarszczona
zamszowa
brak_danych
0
2500
5000
7500
10000
12500
15000
17500
kolor_kapelusza
brązowy
żółty
biały
szary
czerwony
pomarańczowy
zielony
fioletowy
różowy
czarny
jasnobrązowy
niebieski
0
5000
10000
15000
20000
25000
zmienia_kolor_lub_puszcza_mleczko_w_reakcji_na_uszkodzenie
nie_zmienia_koloru_lub_brak_mleczka
zmienia_kolor_lub_puszcza_mleczko
0
10000
20000
30000
40000
50000
sposób_przyrastania_blaszek_do_trzonu
przyrośnięte
zbiegające
wykrojone
rurki
wolne
faliste
brak
brak_danych
0
2000
4000
6000
8000
10000
12000
gęstość_blaszek
gęste
rzadkie
brak
brak_danych
0
5000
10000
15000
20000
25000
kolor_blaszek
biały
brązowy
żółty
różowy
szary
brak
pomarańczowy
czarny
zielony
czerwony
fioletowy
jasnobrązowy
0
2500
5000
7500
10000
12500
15000
17500
podstawa_trzonu
pękaty
bulwiasty
korzeniasty
maczugowaty
brak_danych
0
10000
20000
30000
40000
50000

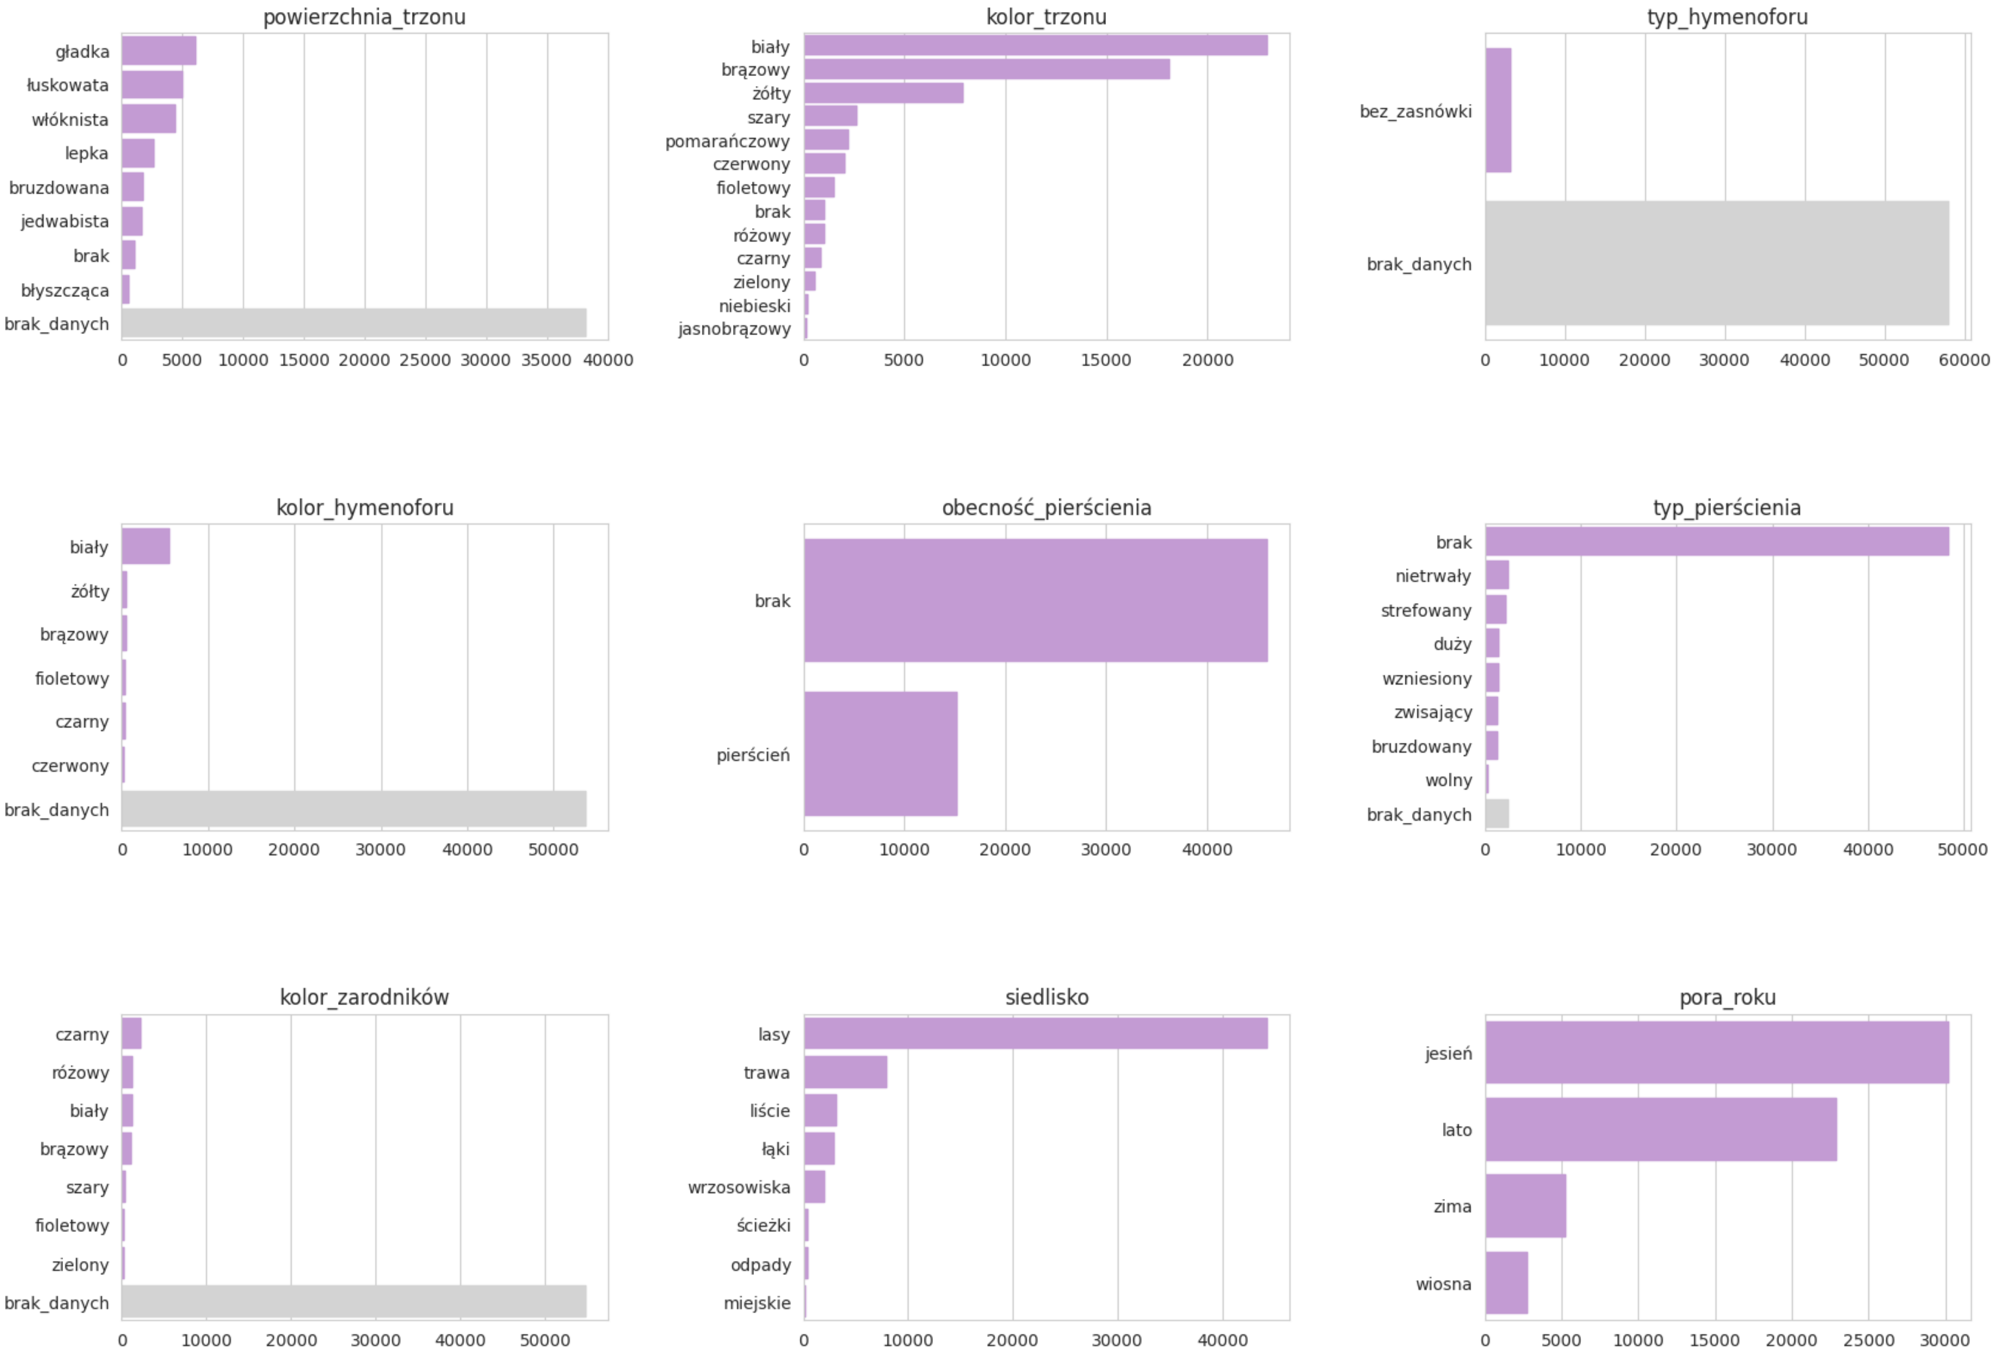
powierzchnia_trzonu
gładka
łuskowata
włóknista
lepka
bruzdowana
jedwabista
brak
błyszcząca
brak_danych
0
5000
10000
15000
20000
25000
30000
35000
40000
kolor_trzonu
biały
brązowy
żółty
szary
pomarańczowy
czerwony
fioletowy
brak
różowy
czarny
zielony
niebieski
jasnobrązowy
0
5000
10000
15000
20000
typ_hymenoforu
bez_zasnówki
brak_danych
0
10000
20000
30000
40000
50000
60000
kolor_hymenoforu
biały
żółty
brązowy
fioletowy
czarny
czerwony
brak_danych
0
10000
20000
30000
40000
50000
obecność_pierścienia
brak
pierścień
0
10000
20000
30000
40000
typ_pierścienia
brak
nietrwały
strefowany
duży
wzniesiony
zwisający
bruzdowany
wolny
brak_danych
0
10000
20000
30000
40000
50000
kolor_zarodników
czarny
różowy
biały
brązowy
szary
fioletowy
zielony
brak_danych
0
10000
20000
30000
40000
50000
siedlisko
lasy
trawa
liście
łąki
wrzosowiska
ścieżki
odpady
miejskie
0
10000
20000
30000
40000
pora_roku
jesień
lato
zima
wiosna
0
5000
10000
15000
20000
25000
30000

Statystyki opisowe:

| | średnica_kapelusza_cm | wysokość_trzonu_cm | szerokość_trzonu_mm |
|---|---|---|---|
| liczba | 61069.00 | 61069.00 | 61069.00 |
| średnia | 6.73 | 6.58 | 12.15 |
| odch. stand. | 5.26 | 3.37 | 10.04 |
| minimum | 0.38 | 0.00 | 0.00 |
| 25% | 3.48 | 4.64 | 5.21 |
| mediana | 5.86 | 5.95 | 10.19 |
| 75% | 8.54 | 7.74 | 16.57 |
| maksimum | 62.34 | 33.92 | 103.91 |

Brakujące dane (liczba i procent):

| Kolumna | Liczba | Procent |
|---|---|---|
| typ_hymenoforu | 57892 | 94.80 |
| kolor_zarodników | 54715 | 89.60 |
| kolor_hymenoforu | 53656 | 87.86 |
| podstawa_trzonu | 52597 | 86.13 |
| powierzchnia_trzonu | 38124 | 62.43 |
| gęstość_blaszek | 25063 | 41.04 |
| powierzchnia_kapelusza | 18552 | 30.38 |
| sposób_przyrastania_blaszek_do_trzonu | 9884 | 16.18 |
| typ_pierścienia | 2471 | 4.05 |
| klasa | 0 | 0.00 |
| kolor_trzonu | 0 | 0.00 |
| siedlisko | 0 | 0.00 |
| obecność_pierścienia | 0 | 0.00 |
| szerokość_trzonu_mm | 0 | 0.00 |
| średnica_kapelusza_cm | 0 | 0.00 |
| wysokość_trzonu_cm | 0 | 0.00 |
| kolor_blaszek | 0 | 0.00 |
| zmienia_kolor_lub_puszcza_mleczko_w_reakcji_na_uszkodzenie | 0 | 0.00 |
| kolor_kapelusza | 0 | 0.00 |
| kształt_kapelusza | 0 | 0.00 |
| pora_roku | 0 | 0.00 |

## "Rój pszczół" – wpływ poszczególnych cech owocnika na predykcję jego jadalności (jadalny/niejadalny lub trujący)

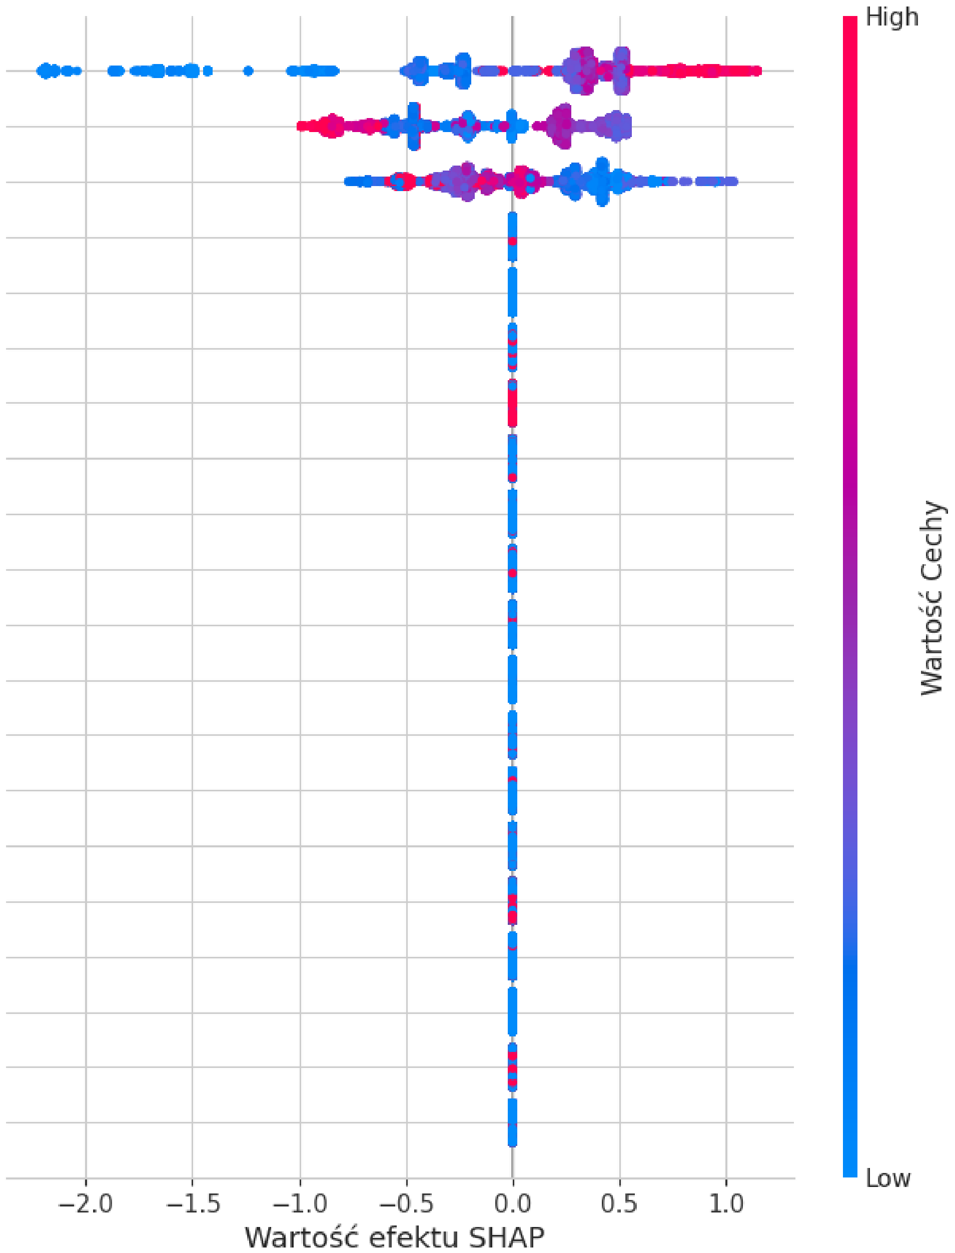


Punkty po prawej (> 0.0) mają większy wpływ na klasyfikację grzyba przez model jako trującego, po lewej jako jadalnego

**Legenda:**

High = wysoka wartość cechy, np. „średnica_kapelusza_cm" (High) = duża średnica kapelusza w cm

Low = niska wartość cechy, np. „wysokość_trzonu_cm" (Low) = krótki trzon

„0" = granica między cechami, które mają duże i małe znaczenie w ocenie jadalności grzyba

Dla cech binarnych (albo jest, albo jej nie ma) wartość wysoka (High), czyli kolor czerwony, oznacza: „cecha jest".

**Wykres „wodospad”: wpływ cech danego owocnika na przewidywanie jego toksyczności**

**Analiza wpływu cech na przewidywanie dla klasy 'niejadalny/trujący' (dla grzyba, który faktycznie jest trujący)**

Wkład poszczególnych cech w przewidywanie klasy grzyba przez model
Wartości pozytywne (w prawo) wskazują na wzrost prawdopodobieństwa klasyfikacji jako „niejadalnego/trującego” wg modelu, wartości negatywne (w lewo) – zmniejszenie
E[f(x)] to średni wynik modelu, a f(X) to przewidywanie dla tej obserwacji

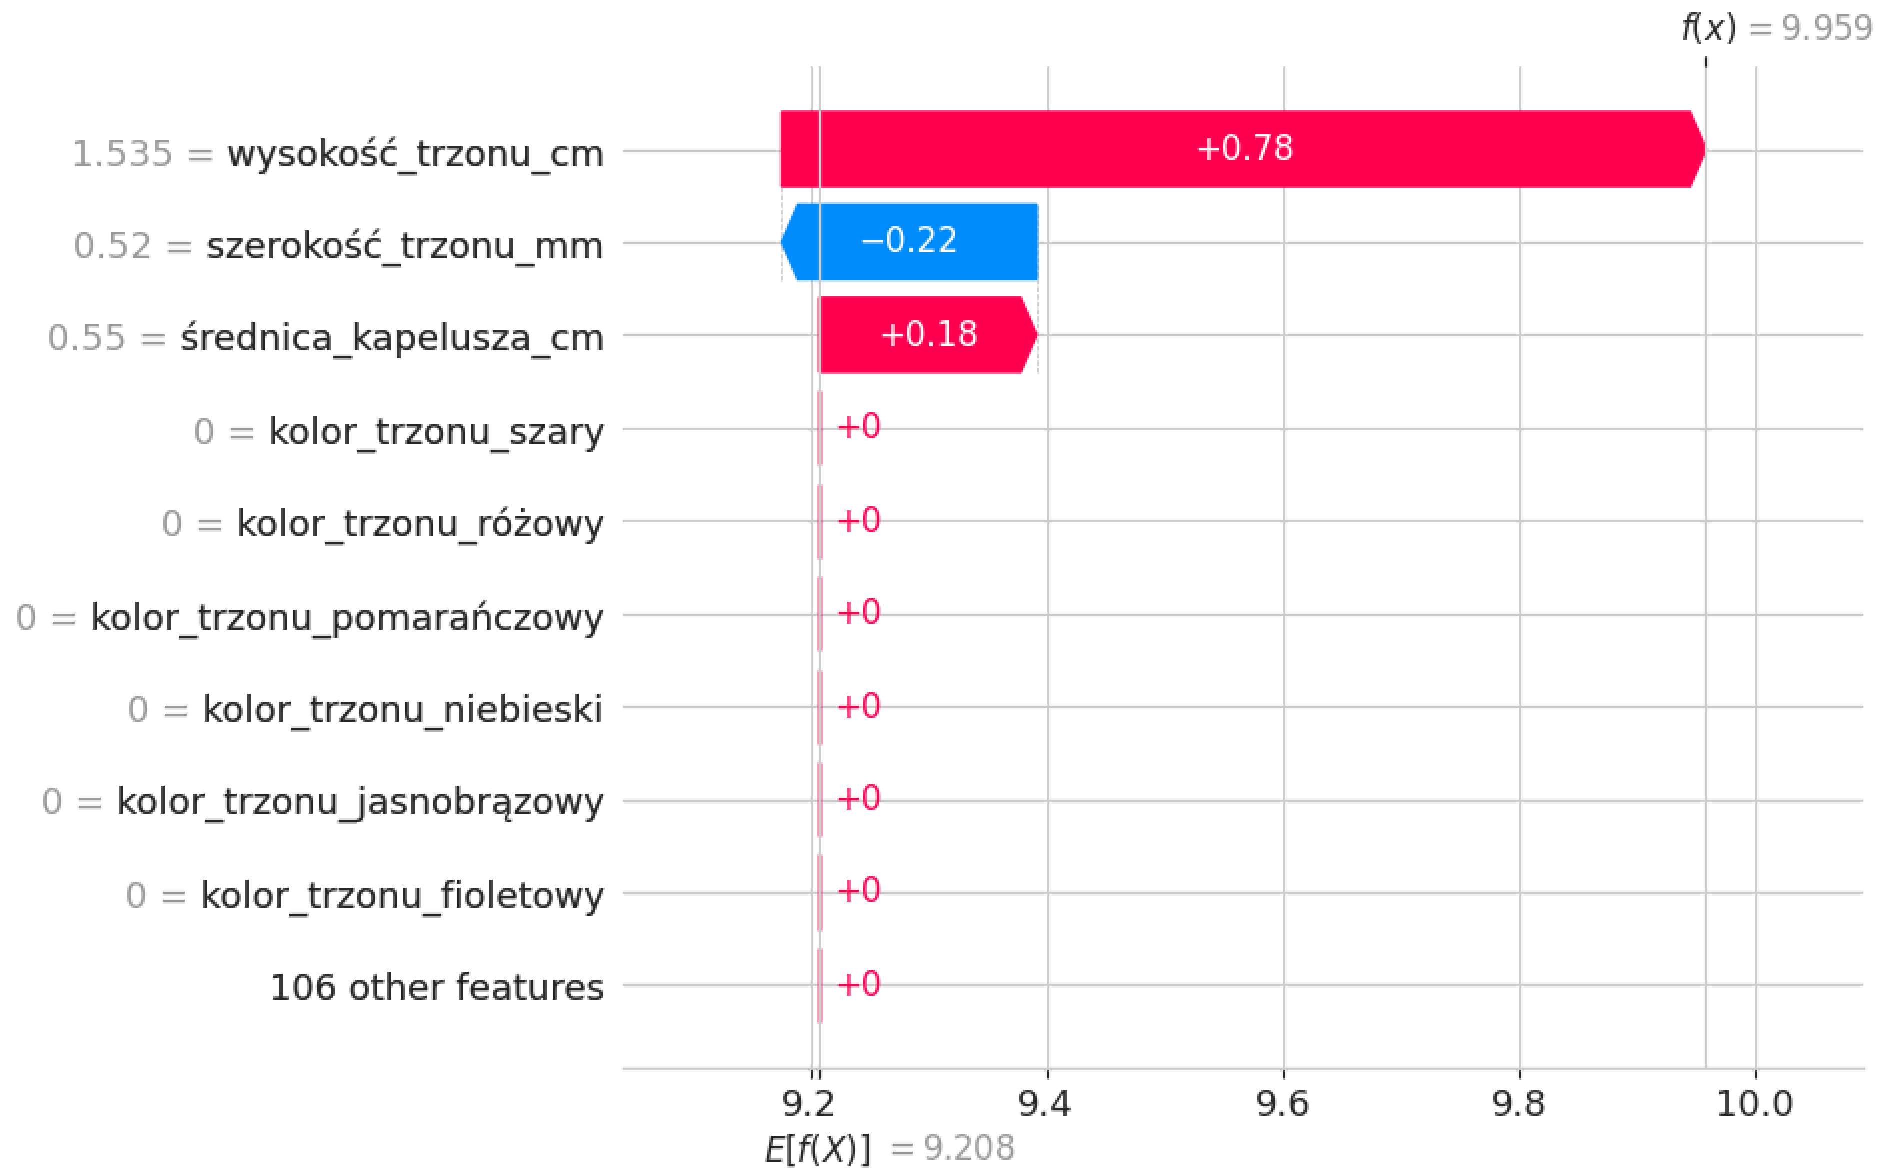


Legenda:

E[f(X)]: wartość bazowa = średnia predykcja modelu dla wszystkich obserwacji

Szarfy kolorowe: wpływ danej cechy na predykcję toksyczności dla konkretnego owocnika

f(x): wartość ostateczna = predykcja modelu dla tego konkretnego owocnika

# Wykres LIME: wartości cech grzybów zmniejszające lub zwiększające prawdopodobieństwo predykcji jadalny/niejadalny lub trujący

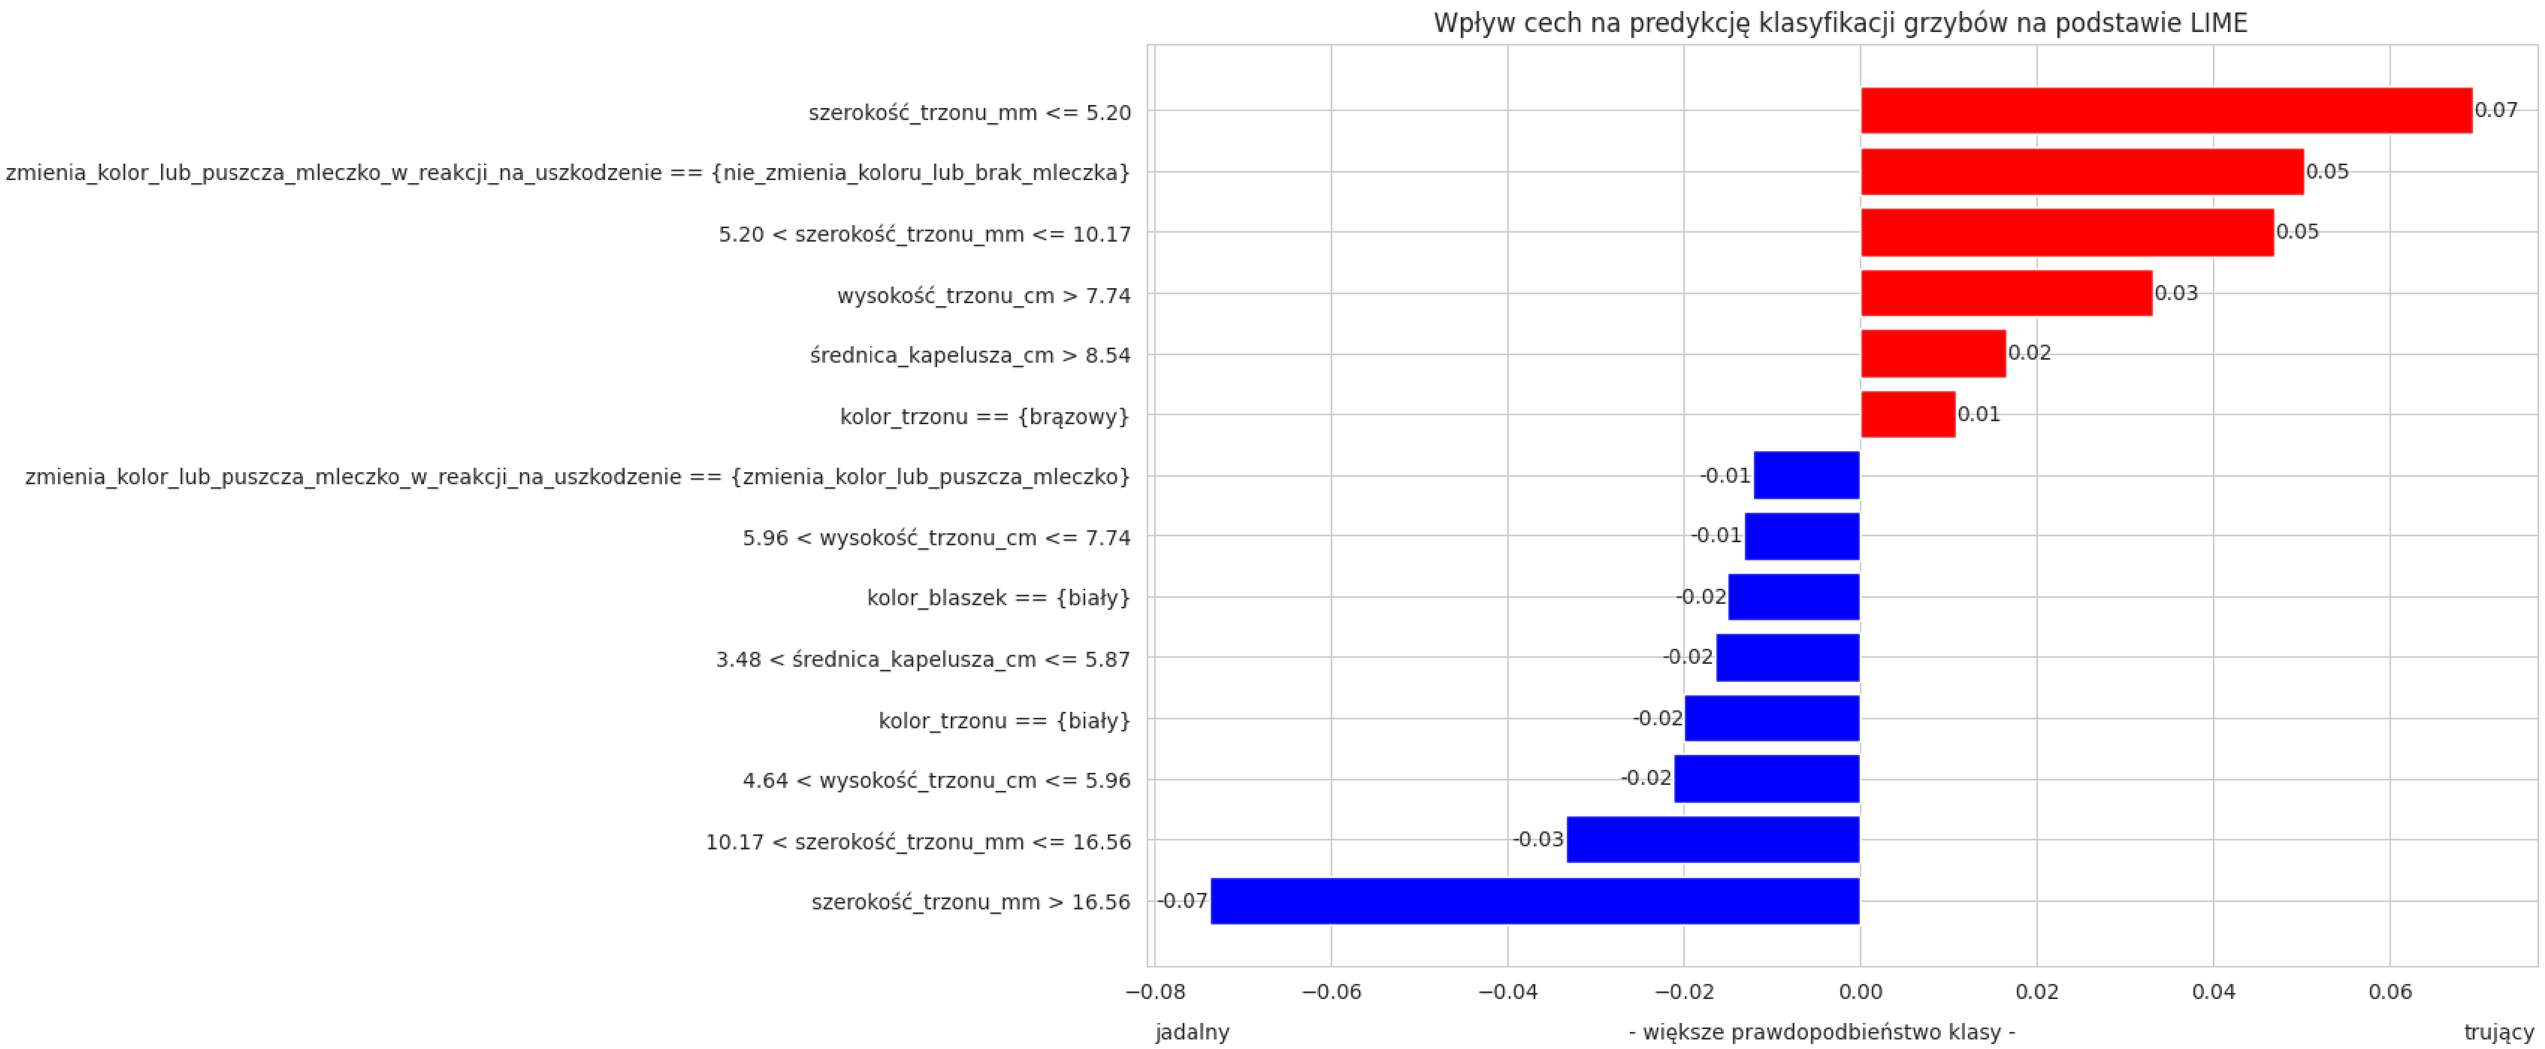

```
Porównanie z obserwacją numer #0:
Cecha                                      Wartość oryginalna                   Wartość zmodyfikowana
----------------------------------------------------------------------------------------------------
  średnica_kapelusza_cm                    9.41
  kształt_kapelusza                        inne
  powierzchnia_kapelusza                   lepka
  kolor_kapelusza                          żółty
  zmienia_kolor_lub_puszcza_
   _mleczko_w_reakcji_na_uszkodzenie   nie_zmienia_koloru_lub_brak_mleczka
  sposób_przyrastania_blaszek_do_trzonu    brak_danych
  gęstość_blaszek                          gęste
  kolor_blaszek                            pomarańczowy
  wysokość_trzonu_cm                       1.43                             ->  23.5
  szerokość_trzonu_mm                      16.03
  podstawa_trzonu                          brak_danych
  powierzchnia_trzonu                      brak_danych
  kolor_trzonu                             brązowy
  typ_hymenoforu                           brak_danych
  kolor_hymenoforu                         brak_danych
  kolor_zarodników                         brak_danych
  siedlisko                                lasy
  pora_roku                                jesień
```

```
Porównanie z obserwacją numer #1:
Cecha                                      Wartość oryginalna                   Wartość zmodyfikowana
----------------------------------------------------------------------------------------------------
  średnica_kapelusza_cm                    9.41
  kształt_kapelusza                        inne
  powierzchnia_kapelusza                   lepka
  kolor_kapelusza                          żółty
  zmienia_kolor_lub_puszcza_
   _mleczko_w_reakcji_na_uszkodzenie   nie_zmienia_koloru_lub_brak_mleczka
  sposób_przyrastania_blaszek_do_trzonu    brak_danych
  gęstość_blaszek                          gęste
  kolor_blaszek                            pomarańczowy
  wysokość_trzonu_cm                       1.43                             ->  23.2
  szerokość_trzonu_mm                      16.03
  podstawa_trzonu                          brak_danych
  powierzchnia_trzonu                      brak_danych
  kolor_trzonu                             brązowy
  typ_hymenoforu                           brak_danych
  kolor_hymenoforu                         brak_danych
  kolor_zarodników                         brak_danych
  siedlisko                                lasy
  pora_roku                                jesień
```

## Analiza kontrfaktyczna: jak uzupełnienie przez AI brakujących danych w opisie konkretnego owocnika wpływa na zmianę predykcji jego jadalności

**Objaśnienie:**
**Opisany na wizualizacji owocnik, badany realnie w przyrodzie, był NIEJADALNY/TRUJĄCY.**
Model AI poprawnie przypisał go do przewidywanej klasy NIEJADALNY/TRUJĄCY.

Dwie przedstawione na obrazie analizy kontrfaktyczne mówią, jakie dane wystarczy zmienić, aby ten owocnik otrzymał predykcję **JADALNY.**

**Legenda:**
Wartość pierwotna: dana pobrana dla konkretnego owocnika z pierwotnego zbioru danych

Wartość zmieniona: dana zmieniona lub uzupełniona przez model AI

W badaniu wykorzystano zaawansowany model uczenia maszynowego, znany jako **Klasyfikator wzmocnienia gradientowego** (w skrócie: “XGBClassifier”). Ten model osiągnął dokładność na poziomie **99,97%**, co świadczy o jego wysokiej skuteczności w odróżnianiu grzybów jadalnych od niejadalnych lub trujących.

**Wysoka dokładność:** Model skutecznie identyfikuje, czy dany grzyb jest jadalny czy niejadalny lub trujący, opierając się na analizie różnych cech owocnika.

**Bazowanie na danych:** Decyzje modelu opierają się wyłącznie na danych, które zostały mu dostarczone. Oznacza to, że model wykorzystuje dostępne informacje do wyciągania wniosków, ale *nie posiada wiedzy poza zakresem tych danych*.

**Ograniczenia modelu:** Chociaż model jest bardzo dokładny, należy pamiętać o jego ograniczeniach. Nie jest on w stanie uwzględnić wszystkich możliwych czynników wpływających na jadalność grzybów, które mogą być znane ekspertom. Model stanowi dodatkowe narzędzie wspomagające identyfikację grzybów. Jednakże, ze względu na ograniczenia modelu, zaleca się, aby nie traktować jego predykcji jako ostatecznego wyznacznika decyzji, a raczej jako jeden z elementów w procesie identyfikacji grzybów.

W naszym badaniu zastosowano standardową metodę podziału danych na dwie grupy: jedną do nauki modelu (zbiór treningowy) i drugą do jego testowania (zbiór testowy).

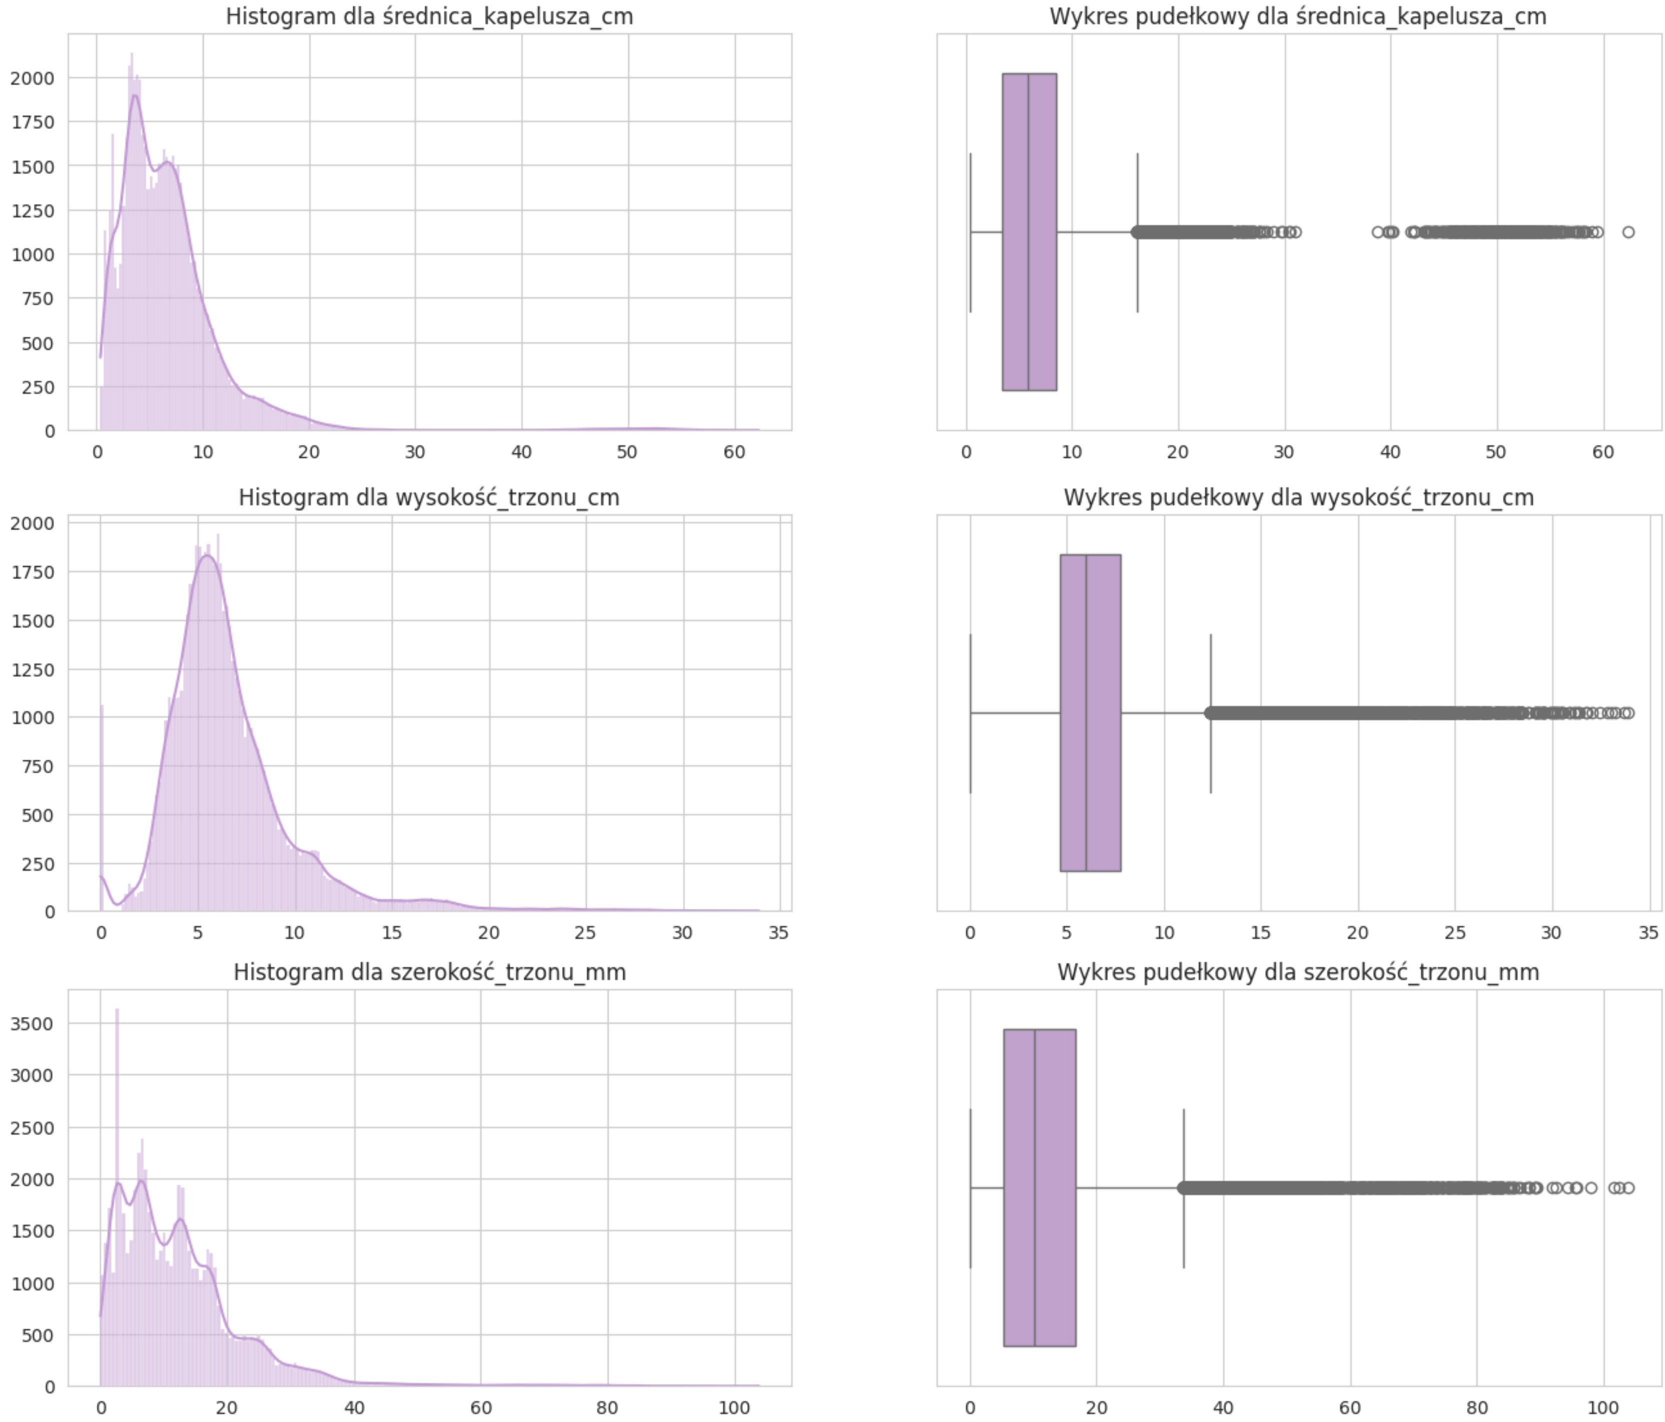
Histogram dla średnica_kapelusza_cm
Wykres pudełkowy dla średnica_kapelusza_cm
Histogram dla wysokość_trzonu_cm
Wykres pudełkowy dla wysokość_trzonu_cm
Histogram dla szerokość_trzonu_mm
Wykres pudełkowy dla szerokość_trzonu_mm

Example Przykład

średnica_kapelusza_cm > 8.54

kształt_kapelusza = wypukły

powierzchnia_kapelusza = gładka

kolor_kapelusza = biały

zmienia_kolor_lub_puszcza_mleczko_w_reakcji_na_uszkodzenie = nie_zmienia_koloru_lub_brak_mleczka

sposób_przyrastania_blaszek_do_trzonu = faliste

gęstość_blaszek = gęste

kolor_blaszek = biały

5.96 < wysokość_trzonu_cm <= 7.74

szerokość_trzonu_mm > 16.56

podstawa_trzonu = brak_danych

powierzchnia_trzonu = brak_danych

kolor_trzonu = biały

typ_hymenoforu = brak_danych

kolor_hymenoforu = brak_danych

kolor_zarodników = brak_danych

siedlisko = łąki

pora_roku = wiosna

^

A.I. prediction Predykcja AI

jadalny

# "KOTWICA" (anchor) - metoda objaśniania modelu AI

Po prawej u góry: kotwica, czyli zestaw cech, których łączna obecność (koniunkcja) przesądza o sposobie zaklasyfikowania danego owocnika przez model AI.
Kotwica nie musi odzwierciedlać rzeczywistego przykładu z danych.

Poniżej kotwicy: wpływ łącznego występowania zestawu cech (kotwicy) na procent przypadków, w których model przewiduje daną klasę (czyli tzw. pewność klasyfikacji).
W wyliczaniu tego procentu model uwzględnia cechy zaznaczone na niebiesko.

Explanation of A.I. prediction Objaśnienie kryteriów predykcji (decyzji) AI

If ALL of these are true: Gdy wszystkie te cechy są spełnione

✓ powierzchnia_trzonu = brak_danych ✓ szerokość_trzonu_mm > 10.17
✓ podstawa_trzonu = brak_danych ✓ powierzchnia_kapelusza = gładka
✓ kolor_trzonu = biały ✓ sposób_przyrastania_blaszek_do_trzonu = faliste
✓ średnica_kapelusza_cm > 5.87 ✓ wysokość_trzonu_cm <= 7.74

The A.I. will predict jadalny 97.2% of the time

AI przewiduje klasę JADALNY w 97,2% przypadków

If ALL of these are true: Gdy wszystkie te cechy są spełnione

✓ powierzchnia_trzonu = brak_danych ✓ szerokość_trzonu_mm > 10.17
✓ podstawa_trzonu = brak_danych ✓ powierzchnia_kapelusza = gładka
✓ kolor_trzonu = biały sposób_przyrastania_blaszek_do_trzonu = faliste
średnica_kapelusza_cm > 5.87 wysokość_trzonu_cm <= 7.74

The A.I. will predict jadalny 76.2% of the time

AI przewiduje klasę JADALNY w 76,2% przypadków

**Example** Przykład

5.87 < średnica_kapelusza_cm <= 8.54

kształt_kapelusza = płaski

powierzchnia_kapelusza = brak_danych

kolor_kapelusza = zielony

zmienia_kolor_lub_puszcza_mleczko_w_reakcji_na_uszkodzenie = nie_zmienia_koloru_lub_brak_mleczka

sposób_przyrastania_blaszek_do_trzonu = wykrojone

gęstość_blaszek = gęste

kolor_blaszek = brązowy

5.96 < wysokość_trzonu_cm <= 7.74

10.17 < szerokość_trzonu_mm <= 16.56

podstawa_trzonu = brak_danych

powierzchnia_trzonu = brak_danych

kolor_trzonu = biały

typ_hymenoforu = brak_danych

kolor_hymenoforu = brak_danych

kolor_zarodników = brak_danych

siedlisko = lasy

pora_roku = jesień

**A.I. prediction** Predykcja AI

trujący

# "KOTWICA" (anchor) - metoda objaśniania modelu AI

Po prawej u góry: kotwica, czyli zestaw cech, których łączna obecność (koniunkcja) przesądza o sposobie zaklasyfikowania danego owocnika przez model AI.
Kotwica nie musi odzwierciedlać rzeczywistego przykładu z danych.

Poniżej kotwicy: wpływ łącznego występowania zestawu cech (kotwicy) na procent przypadków, w których model przewiduje daną klasę (czyli tzw. pewność klasyfikacji).
W wyliczaniu tego procentu model uwzględnia cechy zaznaczone na niebiesko.

**Explanation of A.I. prediction** Objaśnienie kryteriów predykcji (decyzji) AI

If ALL of these are true: Gdy wszystkie te cechy są spełnione

- ✓ sposób_przyrastania_blaszek_do_trzonu = wykrojone
- ✓ kolor_kapelusza = zielony
- ✓ powierzchnia_kapelusza = brak_danych
- ✓ kształt_kapelusza = płaski
- ✓ średnica_kapelusza_cm > 5.87

The A.I. will predict trujący **97.5%** of the time

AI przewiduje klasę TRUJĄCY w 97,5% przypadków

If ALL of these are true: Gdy wszystkie te cechy są spełnione

- ✓ sposób_przyrastania_blaszek_do_trzonu = wykrojone
- ✓ kolor_kapelusza = zielony
- powierzchnia_kapelusza = brak_danych
- kształt_kapelusza = płaski
- średnica_kapelusza_cm > 5.87

The A.I. will predict trujący **84.0%** of the time

AI przewiduje klasę TRUJĄCY w 84,0% przypadków
